# Supplementary material for: High-fidelity software-defined quantum logic on a superconducting qudit
Source: arXiv:2005.13165 source file (2020-10-19)
Supplement: Supplementary file 1 [file wuEtAl_optimalControl_PRL_SM-V3.pdf]

# Supplemental Material: High-fidelity software-defined quantum logic on a superconducting qudit

Xian Wu, S. L. Tomarken, N. Anders Petersson, L. A. Martinez, Yaniv J. Rosen, Jonathan L DuBois
*Lawrence Livermore National Laboratory, Livermore, CA 94550, USA*

## STATE CLASSIFICATION

The state of the qudit is determined by driving the cavity near its resonance with a square pulse of roughly 3 µs duration and measuring the cavity's state-dependent dispersive shift [1]. Figure S1(a) illustrates the cavity's state-dependent shift $\chi_{qc} \simeq 1.017$ MHz. We fix the readout frequency at an optimal point where we obtain the greatest distinguishability in the plane defined by the in-phase ($I$) and quadrature phase ($Q$) of the readout signal. In Fig. S1(b), the four separated clusters represent the four lowest qudit states. To collect this data, we first prepared the qudit in one of its lowest four eigenstates with either a single square pulse or a series of square pulses (or thermal relaxation for the ground state) and subsequently measured the signal in $I-Q$ space. Measurements were repeated 51200 times for each initial state. A total of 204800 $(I,Q)$ pairs are used to establish the histogram in Fig. S1(b).

The data in Fig. S1 forms the basis of our qudit state classifier. Specifically, we assume that all data points are generated from a mixture of four Gaussian distributions, each representing one qudit state. We use the GaussianMixture class from the scikit-learn.mixture python module [2] to build the classifier. Based on the $I-Q$ coordinates of the readout signal, the classifier predicts the probability that it belongs to each state. We assign each data point to the state with the highest probability.

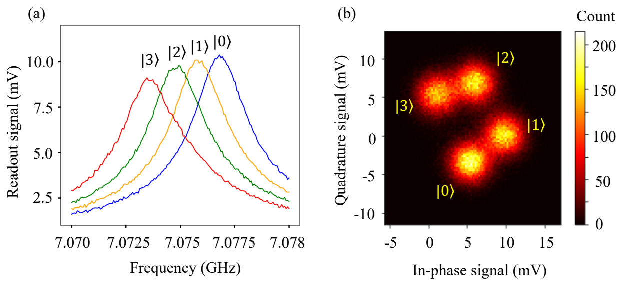


FIG. S1. **Readout of the transmon qudit (a)** State-dependent shifts of the cavity resonance. The cavity shift for adjacent qudit states is approximately 1.017 MHz. **(b)** Histogram of the in-phase ($I$) and quadrature phase ($Q$) signals for the lowest four qudit states.

TABLE S1. Distribution of qudit measurement outcomes for different prepared sates.

| **Prepared state** | **Detected state (%)** | | | |
|---|---|---|---|---|
| | $\|0\rangle$ | $\|1\rangle$ | $\|2\rangle$ | $\|3\rangle$ |
| $\|0\rangle$ | 95.85 | 3.95 | 0.08 | 0.12 |
| $\|1\rangle$ | 8.09 | 90.9 | 0.69 | 0.30 |
| $\|2\rangle$ | 1.95 | 19.99 | 74.08 | 3.98 |
| $\|3\rangle$ | 1.84 | 3.86 | 17.27 | 77.03 |

Next, we use the classifier to examine each prepared state. The detected state distributions for each prepared state are listed in Table S1. For the prepared state $|0\rangle$, we observe roughly 96 % is detected correctly as the $|0\rangle$ state, while 4 % is detected as belonging to one of the other four qudit states. We attribute the 4 % misclassification error to overlap between the constituent Gaussian distributions of each state. $|1\rangle$ is closest to $|0\rangle$, which constitutes most of the 4 % difference. For the excited states, state decay during measurement leads to nontrivial populations of the lower energy states. For example, measurements on prepared $|1\rangle$ states show about 8 % $|0\rangle$ occupation due mainly to $T_1$ decay during the 3 µs measurement pulse in addition to misclassification errors due to Gaussian overlap.

In order to best estimate the measured qudit state, we use Table S1 to construct a *confusion matrix* $P$, which is defined as described in Ref. 3:

$$P = \begin{pmatrix} p(0|0) & p(0|1) & p(0|2) & p(0|3) \\ p(1|0) & p(1|1) & p(1|2) & p(1|3) \\ p(2|0) & p(2|1) & p(2|2) & p(2|3) \\ p(3|0) & p(3|1) & p(3|2) & p(3|3) \end{pmatrix}, \qquad \text{(S1)}$$

where $p(j|k)$ is defined as the probability of detecting the state $|j\rangle$ given the perfect preparation of the initial state $|k\rangle$.

In this treatment, we describe a given quantum state's probability distribution with a column vector of probabilities $\vec{p}$. The matrix $P$ relates the detected outcome probability distribution $\vec{p}_d$ and the actual probability distribution $\vec{p}_{\rm ac}$ of the collapsed quantum state as $\vec{p}_d = P\vec{p}_{\rm ac}$. Taking the inverse of the confusion matrix $P^{-1}$, we can infer the actual qudit probability distribution from the detected probability distribution determined by the classifier. Measurement data shown in Fig. 2 and Fig. 3 of the main text are processed using the methods described above. Due to the instability of the output amplifier at base temperature, the readout signal corresponding to a specific state can itself become unstable over time. This causes a small fraction of our processed data to obtain unphysical probabilities (above 1 or below 0). However, we believe the contribution of the amplifier instability is

not significant and the vast majority of the data accurately describes the underlying physics.

## HAMILTONIAN OF THE QUDIT

We use the charge basis to describe the transmon Hamiltonian. The effective offset charge $n_g$ is measured in units of the Cooper pair charge $2e$. As usual, the full Hamiltonian consists of the electrostatic component $H_{\mathrm{el}}$ and the Josephson component $H_J$:

$$H_T = H_{\mathrm{el}} + H_J \tag{S2}$$

$$H_{\mathrm{el}} = 4E_C\left(\hat{N} - n_g\right)^2 \tag{S3}$$

$$H_J = -\frac{E_J}{2}\sum_n \left(|n\rangle\langle n+1| + |n+1\rangle\langle n|\right) \tag{S4}$$

where $E_C = e^2/2C_\Sigma$ is the electrostatic charging energy to add a single electron to the island with total capacitance $C_\Sigma$, $\hat{N}$ is the number operator (number of Cooper pairs), $E_J = I_c\phi_0/(2\pi)$ is the Josephson energy where $I_c$ is the critical current of the Josephson junction, $\phi_0$ is the flux quantum, and $n$ is the difference in the number of Cooper pairs across the junction.

To solve for the eigenstates, we use a truncated charge basis where $n = -40, -39, \ldots, 0, \ldots, 39, 40$:

$$H_T = \begin{pmatrix} 4E_C\left(-40-n_g\right) & -E_J/2 & 0 & \cdots & 0 \\ -E_J/2 & 4E_C\left(-39-n_g\right) & -E_J/2 & \cdots & 0 \\ \vdots & \vdots & \ddots & \cdots & \vdots \\ 0 & 0 & \cdots & 4E_C\left(39-n_g\right) & -E_J/2 \\ 0 & 0 & \cdots & -E_J/2 & 4E_C\left(40-n_g\right) \end{pmatrix} \tag{S5}$$

with fitting parameters $E_C$ and $E_J$. The calculated eigenenergies of the lowest five states match our measured results well. We extract $E_C \simeq 198.8\,\mathrm{MHz}$, $E_J \simeq 11.67\,\mathrm{GHz}$. The first three transition frequencies of our transmon device and the analogous simulation results are listed in Table S2.

Next, we derive the lowering and raising operators $c, c^\dagger$ in the transmon eigenstate basis. The Cooper-pair number operator in the same truncated charge basis is given by

$$\hat{N} = \begin{pmatrix} -40 & 0 & 0 & \cdots & 0 \\ 0 & -39 & 0 & \cdots & 0 \\ \vdots & \vdots & \ddots & \cdots & \vdots \\ 0 & 0 & \cdots & 39 & 0 \\ 0 & 0 & \cdots & 0 & 40 \end{pmatrix}. \tag{S6}$$

Thus, the matrix elements of $\hat{N}$ in the transmon eigenbasis can be calculated as $\langle i|\hat{N}|j\rangle$. Below we write $\hat{N}$ in the truncated eigenbasis ($N = 4$) of the transmon. Each matrix element is normalized to the $\hat{N}_4^{0,1}$ matrix element.

$$\hat{N}_4 = \begin{pmatrix} 0.0 & 1.0 & 0.0 & -0.033 \\ 1.0 & 0.0 & -1.374 & 0.0 \\ 0.0 & -1.374 & 0.0. & 1.626 \\ -0.033 & 0.0 & 1.626 & 0.0 \end{pmatrix} \tag{S7}$$

where we can define the lowering and raising operators $c, c^\dagger$ for the specific transmon device:

$$c = \begin{pmatrix} 0.0 & 1.0 & 0.0 & -0.033 \\ 0.0 & 0.0 & -1.374 & 0.0 \\ 0.0 & 0.0 & 0.0 & 1.626 \\ 0.0 & 0.0 & 0.0 & 0.0 \end{pmatrix}, \tag{S8}$$

$$c^\dagger = \begin{pmatrix} 0.0 & 0.0 & 0.0 & 0.0 \\ 1.0 & 0.0 & 0.0 & 0.0 \\ 0.0 & -1.374 & 0.0. & 0.0 \\ -0.033 & 0.0 & 1.626 & 0.0 \end{pmatrix}. \tag{S9}$$

TABLE S2. Measured and simulated transmon transition frequencies (GHz)

| | $\|0\rangle \to \|1\rangle$ | $\|1\rangle \to \|2\rangle$ | $\|2\rangle \to \|3\rangle$ |
|---|---|---|---|
| Measured | 4.09948 | 3.87409 | 3.6193 |
| Simulation | 4.09948 | 3.87409 | 3.6242 |

## EXPERIMENTAL SETUP

Figure 1 of the main text shows a schematic of the experimental setup. The drive signal travels down the coaxial cable and is attenuated and filtered before interacting with the qudit. Bandpass filters at the signal input line reduce both low frequency (<1 GHz) and high

frequency (>12 GHz) noise. Homemade Eccosorb CR-110 filters are installed at both input and output ports of the three-dimensional (3D) cavity to reduce infrared radiation entering the cavity. The coaxial cabling and signal line components impose frequency-dependent attenuation. Additionally, the 3D cavity itself functions as a narrow bandpass filter. From the perspective of the qudit, the entire measurement chain can be viewed as a spectral filter on the control signal. In order to faithfully apply the intended control signals, precise knowledge of the frequency-dependent attenuation is required.

### Spectrum filter calibration

In order to calibrate the precise signal amplitude arriving at the qudit, we perform the steps depicted in Fig. S2(a). Starting from the optimized control waveforms in the rotating frame, we convert them into a single waveform in the laboratory frame. Next, we Fourier transform the time-domain control waveform into the frequency domain. There are two main peaks in the frequency domain, each corresponding to one of the qudit transitions as labeled in Fig. S2(c). Because the state $|3\rangle$ is forbidden from occupation during the optimization of the control pulse (through an explicit penalty in the objective function), there is no frequency component related to the $|2\rangle - |3\rangle$ transition.

We adjust the control pulse amplitude for each frequency component according to Fig. S2(d), compensating for the filtering imposed by the measurement chain. Figure S2(d) shows the drive strength for a fixed output amplitude from the arbitrary waveform generator (AWG) as a function of drive frequency. Overall, the drive is attenuated more as the drive frequency decreases. Within a small range of frequency near each qudit transition, the attenuation of the drive is highly nonlinear. Based on the Fourier transform of the control pulse, the frequency components are close to zero everywhere except near the qudit transition frequencies. Therefore, we only measure attenuation of the drive at frequencies near each of the state transitions and linearly interpolate the attenuation elsewhere.

To calculate the attenuation, we apply a cosine waveform with fixed amplitude at frequencies near each qudit transition to induce Rabi oscillations in the time domain. The Rabi oscillation frequency depends on both the detuning of the drive frequency from each qudit transition as well as the drive strength at that particular frequency. For the case of a two-level sytem, there are analytical solutions of the state probabilities [4] as a function of time:

$$P_0(t) = \frac{\mathcal{V}_{01}^2}{\Omega_R^2}\cos^2(\Omega_R t/2) \tag{S10}$$

$$P_1(t) = \frac{\mathcal{V}_{01}^2}{\Omega_R^2}\sin^2(\Omega_R t/2) \tag{S11}$$

$$\Omega_R = \sqrt{\mathcal{V}_{01}^2 + \Delta^2} \tag{S12}$$

$$\mathcal{V}_{01} = \langle 0|\, \hat{V}\, |1\rangle \tag{S13}$$

where $\hat{V}$ is the drive strength, $\mathcal{V}_{01}$ is the coupling strength between the two states being driven, and $\Delta$ is the detuning of the drive from the state transition. $P_0, P_1$ are population of the two states, and they oscillate with rate $\Omega_R$ related to $\mathcal{V}_{01}$ and $\Delta$ according to Eq. S12.

Although we have more than two states, the drive frequency is far detuned from other state transitions and this set of solutions is applicable. Furthermore, we ensure that the drive strength is sufficiently small so as not to induce significant two-photon absorption. Because we are using fixed amplitude,

$$\hat{V} = \xi_0\left(c + c^\dagger\right). \tag{S14}$$

We obtain a relationship between $\mathcal{V}_{12}, \mathcal{V}_{23}$ and $\mathcal{V}_{01}$. Based on the exact form of $c, c^\dagger$, we have:

$$\mathcal{V}_{12} = 1.374 \cdot \mathcal{V}_{01} \tag{S15}$$

$$\mathcal{V}_{23} = 1.626 \cdot \mathcal{V}_{01}. \tag{S16}$$

Figure S2(d) shows the extracted drive strength in MHz. To compensate for this effect, we rescale the drive strength at $\omega_q^{(0,1)}$ and apply the inverse of the relative attenuation factor to all of the frequency components of the pulse.

In the end, the control waveform is calculated units of Rabi strength (MHz) and must be converted to voltage and uploaded to the AWG for waveform generation. The conversion from MHz to V is determined by driving at a frequency $\omega_d = \omega_q^{0,1}$ at 250 mV on the AWG and observing the Rabi strength to be 6.042 MHz. Therefore, we obtain the conversion factor from MHz to V to be 0.0414 V/MHz.

Several aspects of our optimal control scheme can be improved to further reduce the gate error. The accuracy and resolution of our current spectral filter can be improved by using a multi-state Rabi model to predict the drive strength for each frequency component. Additionally, we have observed that the AWG itself has a significant nonlinear output as a function of the drive amplitude. Careful characterization of the AWG output and applying appropriate compensation in software would guarantee more faithful implementation of the intended control waveform. Increasing the qudit drive coupling strength can reduce the error arising from qudit decoherence by allowing a shorter total gate time.

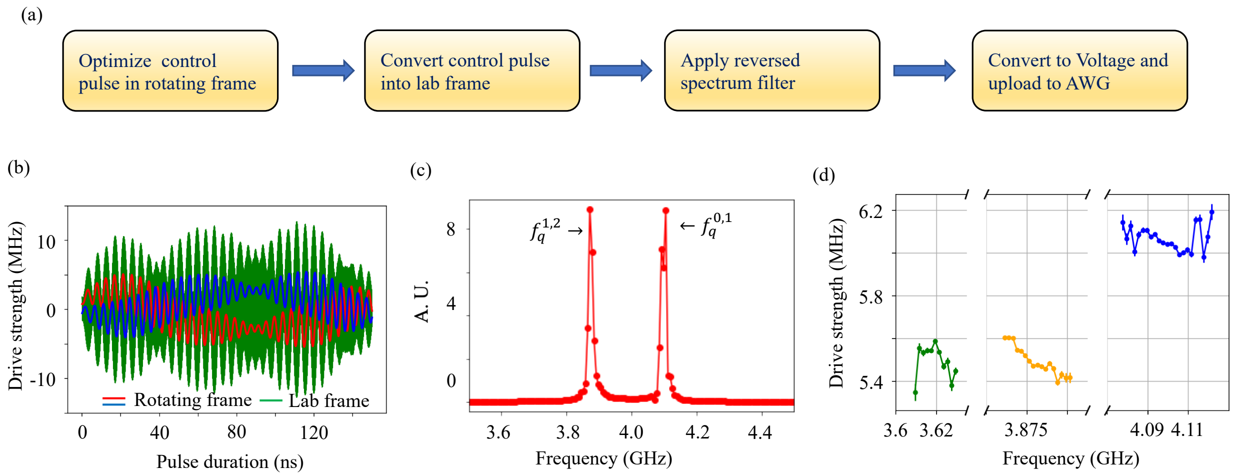


FIG. S2. **Spectrum filter calibration procedure (a)** Flow chart of the main steps required to compensate for frequency-dependent filtering of the measurement chain. **(b)** Calculated control pulse of the $0 \leftrightarrow 2$ SWAP gate. The slowly varying traces are the real and imaginary component of the control pulse in the rotating frame. The rapidly oscillating trace is the control pulse in laboratory frame. **(c)** Fast Fourier Transform of the control functions in the laboratory frame. **(d)** Drive strength with fixed drive amplitude as a function of the drive frequency.

## SIMULATION RESULTS OF THE REPEATED-GATE MEASUREMENT

Figure S3 shows the QuTiP master equation simulation results of the ideal gate with typical values of $T_1$ and $T_2$. The gate is repeated up to 21 times. The simulation qualitatively agrees with our measurement results, see Fig. 2(a)–(d) in the main text.

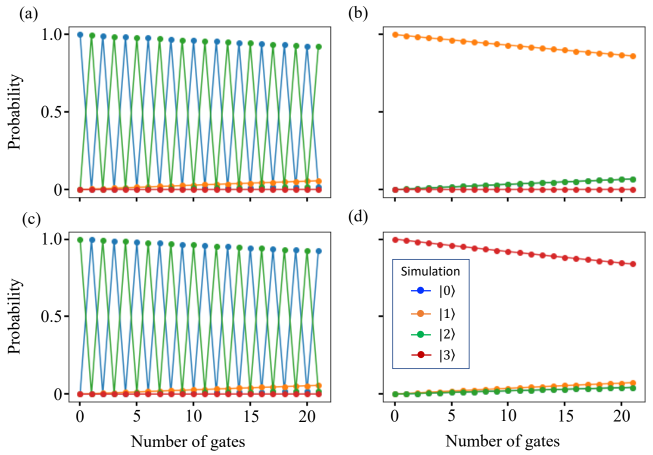


FIG. S3. **Simulation of ideal gate with realistic device decay and decoherence parameters (a)–(d)** The qudit is initialized in $|0\rangle, |1\rangle, |2\rangle, |3\rangle$, respectively.

## ESTIMATING THE PROCESS MATRIX

A quantum operation is a linear map $\rho \rightarrow \mathcal{E}(\rho)$ which completely describes the dynamics of a quantum system. It is convenient to describe $\mathcal{E}(\rho)$ using a fixed set of operators $B_i$ which form a basis for the quantum operation on the same state space.

$$\mathcal{E}(\rho) = \sum_{m,n=0}^{d^2-1} \chi_{mn} B_m \rho B_n^\dagger \tag{S17}$$

$$\begin{aligned} B_i = \{&I, Z_{01}, Z_{12}, \\ &X_{01}, X_{12}, Y_{01}, Y_{12} \\ &X_{01}X_{12}, X_{12}X_{01}\} \end{aligned} \tag{S18}$$

where $\chi$ is a positive Hermitian matrix and depends on the specific gate basis $B_i$ which is not unique. The completeness relation is enforced by

$$\sum_{m,n=0}^{d^2-1} \chi_{mn} B_m^\dagger B_n = I. \tag{S19}$$

We now describe the procedures to estimate $\chi$ with the chosen $B_i$ through our repeated-gate results described in the main text. We first write the process matrix in a Cholesky decomposition to ensure that $\chi$ is Hermitian:

$$\chi([t]) = L^\dagger([t]) L([t]) \tag{S20}$$

where $L$ is a lower-triangular matrix parameterized by a list of variable $[t]$:

$$L\left([t]\right) = \begin{bmatrix} t_0 & 0 & 0 & \cdots & 0 \\ t_1 & t_2 & 0 & \cdots & 0 \\ t_3 & t_4 & t_5 & \cdots & 0 \\ \vdots & \vdots & \vdots & \ddots & \vdots \\ t_{36} & t_{37} & t_{38} & \cdots & t_{44} \end{bmatrix} + i \begin{bmatrix} 0 & 0 & 0 & \cdots & 0 \\ t_{45} & 0 & 0 & \cdots & 0 \\ t_{46} & t_{47} & 0 & \cdots & 0 \\ \vdots & \vdots & \vdots & \ddots & \vdots \\ t_{72} & t_{73} & t_{74} & \cdots & t_{80} \end{bmatrix}. \tag{S21}$$

Next, we apply the mapping defined in Eq. S17 to the initial states $|0\rangle, |1\rangle, |2\rangle$ repeatedly up to 21 times to generate a list of $\rho_n^{0,1,2}$. We compare our measured state occupation probabilities after each gate application to the diagonal elements of each $\rho_n^{0,1,2}$. We fit for the $[t]$ that minimizes the objective function:

$$f([t]) = \sum_{i,k=0}^{2} \sum_{n=1}^{21} \left[m_{i,k,n} - \rho^{i}_{n,kk}\right]^2 \tag{S22}$$

where $m$ represents measurement results and subscripts $i$ indicates the initial states, $n$ represents the number of gate applications, and $kk$ represents the diagonal elements of each density matrix. Minimizing an objective function with 81 variables is very computationally expensive. Additionally, there may be many local minima in the relevant parameter space. Because our single gate application result agrees well with our simulation, we believe that the actual process is very close to the target operator. We extract the $[t]$ that corresponds to the $U_{\text{targ}}$ and use this $[t]$ as the initial guess to minimize the objective function. To satisfy the completeness relation, we add the constrain given by Eq. S19 to the minimization problem. We use the minimize function from the scipy.optimize python module (using method 'SLSQP'). Later, we plot the simulated state probability using the estimate $\chi$ alongside measurement results for comparison.

To measure how closely the quantum dynamics approximates the target dynamics, we calculate the entanglement and gate fidelity defined in Eqs. 8–9 in the main text. We generate 1000 random states $\rho$ and calculate the entanglement fidelity for each one. A distribution of the entanglement fidelity is plotted in Fig. S4(a) from which we obtain an average fidelity of 99.2 %. To estimate the averaged gate fidelity, we generate gate fidelity distribution for 1000 random state vectors $|\psi\rangle$. Results are shown in Fig. S4(b), from which we acquire averaged gate fidelity of 99.4%.

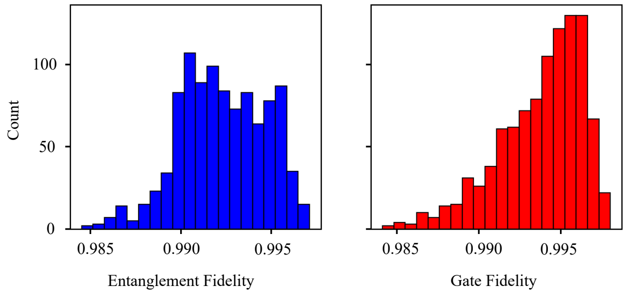


FIG. S4. **Distributions of fidelities (a)** Entanglement fidelity **(b)** Gate fidelity

[1] A. Blais, R.-S. Huang, A. Wallraff, S. M. Girvin, and R. J. Schoelkopf, Physical Review A **69**, 062320 (2004).

[2] F. Pedregosa, G. Varoquaux, A. Gramfort, V. Michel, B. Thirion, O. Grisel, M. Blondel, P. Prettenhofer, R. Weiss, V. Dubourg, J. Vanderplas, A. Passos, D. Cournapeau, M. Brucher, M. Perrot, and E. Duchesnay, Journal of Machine Learning Research **12**, 2825 (2011).

[3] M. Reagor, C. B. Osborn, N. Tezak, A. Staley, G. Prawiroatmodjo, *et al.*, Science Advances **4**, eaao3603 (2018).

[4] C. Gerry and P. Knight, *Introductory Quantum Optics* (Cambridge University Press, 2004).
